# Supplementary material for: Extension of the Active-Orbital-Based and Adaptive CC($P$;$Q$) Approaches to Excited Electronic States: Application to Potential Cuts of Water
Source: arXiv:2411.11245 ancillary file (2024-12-20)
Supplement: Supplementary file 1 [file supplementary_data.pdf]

# Supplementary Data for
# Extension of the Active-Orbital-Based and Adaptive CC($P$;$Q$) Approaches to Excited Electronic States: Application to Potential Cuts of Water

Karthik Gururangan[a], Jun Shen[a], Piotr Piecuch[a,b,*]

[a]*Department of Chemistry, Michigan State University, East Lansing, Michigan 48824, USA*
[b]*Department of Physics and Astronomy, Michigan State University, East Lansing, Michigan 48824, USA*

---

This Supplementary Data document contains the results of the CC and EOMCC calculations for the ground- and excited-state PES cuts of the water molecule, as described by the TZ basis set of Ref. [S1], corresponding to the $H_2O \to H + OH$ dissociation, performed in the present study, along with the associated full CI data taken from Refs. [S1, S2]. Table S1 compares the results of the CCSDT and EOMCCSDT calculations with full CI. The remaining Tables S2 – S13 compare the energies of the ground and excited states of water considered in this work obtained with the CCSD/EOMCCSD, CR-CC(2,3)/CR-EOMCC(2,3), CCSDt/EOMCCSDt, CC(t;3), and adaptive CC($P$;$Q$) approaches for the selected values of the O–H bond-breaking coordinate defining the $H_2O \to H + OH$ dissociation pathway with the parent CCSDT/EOMCCSDT data.

## References

(S1) X. Li, J. Paldus, Performance of multireference and equation-of-motion coupled-cluster methods for potential energy surfaces of low-lying excited states: Symmetric and asymmetric dissociation of water, J. Chem. Phys. 133 (2010) 024102. doi:10.1063/1.3451074.

(S2) J. J. Lutz, P. Piecuch, Performance of the completely renormalized equation-of-motion coupled-cluster method in calculations of excited-state potential cuts of water, Comput. Theor. Chem. 1040–1041 (2014) 20–34. doi:10.1016/j.comptc.2014.05.008.

*Corresponding author
*Email address:* piecuch@chemistry.msu.edu (Piotr Piecuch)

**Table S1**

The CCSDT/EOMCCSDT and full CI total electronic energies for the ground and excited states of the water molecule, as described by the TZ basis set of Ref. [S1], examined in the present study, along the O–H bond-breaking coordinate, $R_{OH}$, in bohr, corresponding to the $H_2O \rightarrow H + OH$ dissociation on the ground-state PES. All energies are shifted by 75 hartree (i.e., reported as $E$ + 75 hartree). The values in parentheses are errors in the CCSDT/EOMCCSDT energies relative to full CI, in millihartree. With the exception of the $3\,{}^3A''$ state, all full CI data were taken from Ref. [S1]. The full CI energies for the $3\,{}^3A''$ state were taken from Ref. [S2]. The lowest-energy orbital correlating with the 1s shell of oxygen was kept frozen in post-RHF calculations.

| | $X\,{}^1A'$ | | $1\,{}^1A''$ | | $1\,{}^3A'$ | |
|---|---|---|---|---|---|---|
| $R_{OH}$ | Full CI | CCSDT | Full CI | EOMCCSDT | Full CI | EOMCCSDT |
| 1.3 | −1.01567 | −1.015602 (0.07) | −0.70187 | −0.702504 (−0.63) | −0.65020 | −0.650784 (−0.58) |
| 1.6 | −1.14894 | −1.148832 (0.11) | −0.85127 | −0.851860 (−0.59) | −0.79340 | −0.793913 (−0.51) |
| 1.809[a] | −1.16847 | −1.168316 (0.15) | −0.88566 | −0.886181 (−0.52) | −0.82511 | −0.825513 (−0.40) |
| 2.0 | −1.16417 | −1.163964 (0.21) | −0.90098 | −0.901368 (−0.39) | −0.84272 | −0.842928 (−0.21) |
| 2.4 | −1.13058 | −1.130217 (0.36) | −0.92945 | −0.929326 (0.12) | −0.89158 | −0.891420 (0.16) |
| 2.8 | −1.09255 | −1.091972 (0.58) | −0.95679 | −0.956186 (0.60) | −0.93780 | −0.937554 (0.25) |
| 3.2 | −1.06129 | −1.060470 (0.82) | −0.97626 | −0.975300 (0.96) | −0.96789 | −0.967653 (0.24) |
| 3.6 | −1.03889 | −1.037848 (1.04) | −0.98862 | −0.987453 (1.17) | −0.98540 | −0.985183 (0.22) |
| 4.0 | −1.02451 | −1.023323 (1.19) | −0.99617 | −0.994949 (1.22) | −0.99516 | −0.994978 (0.18) |
| 4.2 | −1.01967 | −1.018463 (1.21) | −0.99870 | −0.997508 (1.19) | −0.99822 | −0.998050 (0.17) |
| 4.4 | −1.01603 | −1.014832 (1.20) | −1.00065 | −0.999498 (1.15) | −1.00046 | −1.000308 (0.15) |

| | $1\,{}^3A''$ | | $1\,{}^1A'$ | | $2\,{}^3A'$ | |
|---|---|---|---|---|---|---|
| $R_{OH}$ | Full CI | EOMCCSDT | Full CI | EOMCCSDT | Full CI | EOMCCSDT |
| 1.3 | −0.72170 | −0.722266 (−0.57) | −0.62821 | −0.628899 (−0.69) | −0.55577 | −0.556467 (−0.70) |
| 1.6 | −0.87187 | −0.872393 (−0.52) | −0.77055 | −0.771190 (−0.64) | −0.70873 | −0.709251 (−0.53) |
| 1.809[a] | −0.90726 | −0.907714 (−0.45) | −0.79860 | −0.799146 (−0.55) | −0.74823 | −0.748568 (−0.34) |
| 2.0 | −0.92363 | −0.923946 (−0.32) | −0.80575 | −0.806139 (−0.39) | −0.76263 | −0.762831 (−0.20) |
| 2.4 | −0.95148 | −0.951300 (0.18) | −0.81062 | −0.810399 (0.22) | −0.78565 | −0.785421 (0.23) |
| 2.8 | −0.97420 | −0.973528 (0.67) | −0.81932 | −0.818515 (0.81) | −0.81625 | −0.815525 (0.73) |
| 3.2 | −0.98837 | −0.987281 (1.09) | −0.82860 | −0.827420 (1.18) | −0.83261 | −0.831462 (1.15) |
| 3.6 | −0.99640 | −0.995001 (1.40) | −0.83618 | −0.834787 (1.39) | −0.84103 | −0.839577 (1.45) |
| 4.0 | −1.00091 | −0.999363 (1.55) | −0.84172 | −0.840275 (1.44) | −0.84553 | −0.843920 (1.61) |
| 4.2 | −1.00236 | −1.000790 (1.57) | −0.84379 | −0.842366 (1.42) | −0.84693 | −0.845298 (1.63) |
| 4.4 | −1.00345 | −1.001888 (1.56) | −0.84546 | −0.844080 (1.38) | −0.84797 | −0.846350 (1.62) |

| | $2\,{}^3A''$ | | $2\,{}^1A'$ | | $2\,{}^1A''$ | |
|---|---|---|---|---|---|---|
| $R_{OH}$ | Full CI | EOMCCSDT | Full CI | EOMCCSDT | Full CI | EOMCCSDT |
| 1.3 | −0.62356 | −0.624198 (−0.64) | −0.54185 | −0.542618 (−0.77) | −0.61400 | −0.614700 (−0.70) |
| 1.6 | −0.78052 | −0.781036 (−0.52) | −0.68730 | −0.687943 (−0.64) | −0.76861 | −0.769204 (−0.59) |
| 1.809[a] | −0.82109 | −0.821469 (−0.38) | −0.71786 | −0.718367 (−0.51) | −0.80694 | −0.807409 (−0.47) |
| 2.0 | −0.83571 | −0.835975 (−0.26) | −0.72455 | −0.724899 (−0.35) | −0.81992 | −0.820292 (−0.37) |
| 2.4 | −0.82785 | −0.828038 (−0.19) | −0.71631 | −0.716154 (0.16) | −0.81008 | −0.810444 (−0.36) |
| 2.8 | −0.80175 | −0.801866 (−0.12) | −0.72567 | −0.724539 (1.13) | −0.78177 | −0.782217 (−0.45) |
| 3.2 | −0.77863 | −0.778512 (0.12) | −0.73203 | −0.730092 (1.94) | −0.75430 | −0.754820 (−0.52) |
| 3.6 | −0.76634 | −0.765773 (0.57) | −0.73289 | −0.730473 (2.42) | −0.73276 | −0.733362 (−0.60) |
| 4.0 | −0.76393 | −0.763214 (0.72) | −0.72999 | −0.727678 (2.31) | −0.71846 | −0.719183 (−0.72) |
| 4.2 | −0.76335 | −0.762712 (0.64) | −0.72738 | −0.725296 (2.08) | −0.71372 | −0.714539 (−0.82) |
| 4.4 | −0.76232 | −0.761785 (0.54) | −0.72415 | −0.722336 (1.81) | −0.71037 | −0.711300 (−0.93) |

| | $3\,{}^3A''$ | | $3\,{}^1A'$ | | $3\,{}^3A'$ | |
|---|---|---|---|---|---|---|
| $R_{OH}$ | Full CI | EOMCCSDT | Full CI | EOMCCSDT | Full CI | EOMCCSDT |
| 1.3 | −0.36985 | −0.370374 (−0.52) | −0.39097 | −0.391520 (−0.55) | −0.44370 | −0.444133 (−0.43) |
| 1.6 | −0.51578 | −0.516222 (−0.45) | −0.57861 | −0.578996 (−0.39) | −0.61947 | −0.619787 (−0.32) |
| 1.809[a] | −0.55368 | −0.554100 (−0.42) | −0.63701 | −0.637243 (−0.23) | −0.67629 | −0.676486 (−0.20) |
| 2.0 | −0.58208 | −0.582672 (−0.59) | −0.66800 | −0.668055 (−0.05) | −0.71482 | −0.714899 (−0.08) |
| 2.4 | −0.60132 | −0.602051 (−0.73) | −0.69672 | −0.696531 (0.19) | −0.73737 | −0.737345 (0.03) |
| 2.8 | −0.65695 | −0.655011 (1.94) | −0.67863 | −0.678272 (0.36) | −0.70581 | −0.705526 (0.28) |
| 3.2 | −0.69947 | −0.698187 (1.28) | −0.66287 | −0.661466 (1.40) | −0.67660 | −0.675863 (0.74) |
| 3.6 | −0.71715 | −0.716719 (0.43) | −0.66382 | −0.660620 (3.20) | −0.65564 | −0.654127 (1.51) |
| 4.0 | −0.71837 | −0.718451 (−0.08) | −0.66878 | −0.665985 (2.80) | −0.64297 | −0.640046 (2.92) |
| 4.2 | −0.71706 | −0.717253 (−0.19) | −0.66943 | −0.665657 (3.77) | −0.63921 | −0.635295 (3.92) |
| 4.4 | −0.71581 | −0.716073 (−0.26) | −0.66889 | −0.664958 (3.93) | −0.63687 | −0.631806 (5.06) |

[a] The equilibrium value of the O–H bond length in the ground electronic state of water, as obtained in Ref. [S1] using the CCSD/cc-pVTZ method.

**Table S2**

The total electronic energies, reported as errors relative to CCSDT in millihartree, obtained with the CCSD, CR-CC(2,3), CCSDt, CC(t;3), and adaptive CC($P$;$Q$) approaches for the $X\ ^1A'$ state of the water molecule, as described by the TZ basis set of Ref. [S1], along the O–H bond-breaking coordinate, $R_{OH}$, in bohr. The lowest-energy orbital correlating with the 1s shell of oxygen was kept frozen in post-RHF steps.

| | | | | | %T = 1[d] | | %T = 2[e] | |
|---|---|---|---|---|---|---|---|---|
| $R_{OH}$ | CCSD | CR(2,3)[a] | CCSDt[b] | CC(t;3)[c] | CC($P$) | CC($P$;$Q$) | CC($P$) | CC($P$;$Q$) |
| 1.3 | 2.771 | −0.226 | 2.068 | −0.182 | 1.696 | −0.163 | 1.374 | −0.133 |
| 1.6 | 3.063 | −0.269 | 2.229 | −0.205 | 1.713 | −0.171 | 1.331 | −0.124 |
| 1.809[f] | 3.307 | −0.298 | 2.317 | −0.216 | 1.857 | −0.196 | 1.390 | −0.144 |
| 2.0 | 3.562 | −0.325 | 2.361 | −0.219 | 2.141 | −0.230 | 1.652 | −0.175 |
| 2.4 | 4.230 | −0.398 | 2.328 | −0.206 | 2.689 | −0.335 | 2.132 | −0.258 |
| 2.8 | 5.150 | −0.500 | 2.187 | −0.178 | 2.768 | −0.379 | 2.087 | −0.284 |
| 3.2 | 6.389 | −0.613 | 2.023 | −0.151 | 2.575 | −0.369 | 1.898 | −0.275 |
| 3.6 | 7.929 | −0.724 | 1.872 | −0.130 | 2.338 | −0.350 | 1.667 | −0.231 |
| 4.0 | 9.622 | −0.828 | 1.753 | −0.116 | 2.115 | −0.308 | 1.469 | −0.195 |
| 4.2 | 10.448 | −0.875 | 1.709 | −0.112 | 2.043 | −0.276 | 1.405 | −0.183 |
| 4.4 | 11.224 | −0.918 | 1.674 | −0.110 | 1.997 | −0.247 | 1.374 | −0.162 |

[a] CR-CC(2,3) calculations.
[b] CCSDt calculations using the active space consisting of the three highest occupied and two lowest unoccupied RHF orbitals.
[c] CC(t;3) calculations using the active space consisting of the three highest occupied and two lowest unoccupied RHF orbitals.
[d] CC($P$) and CC($P$;$Q$) calculations using $P$ spaces consisting of all singly and doubly excited determinants and 1% of triply excited determinants identified by the adaptive CC($P$;$Q$) algorithm.
[e] CC($P$) and CC($P$;$Q$) calculations using $P$ spaces consisting of all singly and doubly excited determinants and 2% of triply excited determinants identified by the adaptive CC($P$;$Q$) algorithm.
[f] The equilibrium value of the O–H bond length in the ground electronic state of water, as obtained in Ref. [S1] using the CCSD/cc-pVTZ method.

**Table S3**

The total electronic energies, reported as errors relative to EOMCCSDT in millihartree, obtained with the EOMCCSD, CR-EOMCC(2,3), EOMCCSDt, CC(t;3), and adaptive CC($P$;$Q$) approaches for the $1\ ^1A''$ state of the water molecule, as described by the TZ basis set of Ref. [S1], along the O–H bond-breaking coordinate, $R_{OH}$, in bohr. The lowest-energy orbital correlating with the 1s shell of oxygen was kept frozen in post-RHF steps.

| | | | | | %T = 1[d] | | %T = 2[e] | |
|---|---|---|---|---|---|---|---|---|
| $R_{OH}$ | EOMCCSD | CR(2,3)[a] | EOMCCSDt[b] | CC(t;3)[c] | EOMCC($P$) | CC($P$;$Q$) | EOMCC($P$) | CC($P$;$Q$) |
| 1.3 | −0.081 | 0.917 | 1.601 | 0.708 | 2.404 | 0.615 | 2.049 | 0.549 |
| 1.6 | 0.049 | 1.125 | 1.661 | 0.718 | 2.458 | 0.612 | 1.983 | 0.595 |
| 1.809[f] | 0.301 | 1.145 | 1.710 | 0.702 | 2.573 | 0.656 | 2.124 | 0.587 |
| 2.0 | 1.015 | 1.005 | 1.794 | 0.648 | 2.943 | 0.700 | 2.480 | 0.660 |
| 2.4 | 4.319 | 0.505 | 1.972 | 0.485 | 3.802 | 0.620 | 3.093 | 0.534 |
| 2.8 | 7.904 | −0.067 | 1.873 | 0.443 | 3.944 | 0.587 | 2.802 | 0.527 |
| 3.2 | 10.917 | −0.875 | 1.705 | 0.480 | 3.973 | 0.696 | 2.569 | 0.574 |
| 3.6 | 13.263 | −1.810 | 1.594 | 0.537 | 3.637 | 0.869 | 2.261 | 0.681 |
| 4.0 | 14.933 | −2.700 | 1.542 | 0.595 | 3.130 | 0.934 | 1.935 | 0.686 |
| 4.2 | 15.537 | −3.095 | 1.531 | 0.623 | 2.889 | 1.021 | 1.897 | 0.725 |
| 4.4 | 16.012 | −3.448 | 1.527 | 0.649 | 2.995 | 0.999 | 1.789 | 0.725 |

[a] CR-EOMCC(2,3) calculations.
[b] EOMCCSDt calculations using the active space consisting of the three highest occupied and two lowest unoccupied RHF orbitals.
[c] CC(t;3) calculations using the active space consisting of the three highest occupied and two lowest unoccupied RHF orbitals.
[d] EOMCC($P$) and CC($P$;$Q$) calculations using $P$ spaces consisting of all singly and doubly excited determinants and 1% of triply excited determinants identified by the adaptive CC($P$;$Q$) algorithm.
[e] EOMCC($P$) and CC($P$;$Q$) calculations using $P$ spaces consisting of all singly and doubly excited determinants and 2% of triply excited determinants identified by the adaptive CC($P$;$Q$) algorithm.
[f] The equilibrium value of the O–H bond length in the ground electronic state of water, as obtained in Ref. [S1] using the CCSD/cc-pVTZ method.

**Table S4**
Same as Table S3 for the 1 $^3$A′ state.

| | | | | | %T = 1[d] | | %T = 2[e] | |
|---|---|---|---|---|---|---|---|---|
| $R_{\mathrm{OH}}$ | EOMCCSD | CR(2,3)[a] | EOMCCSDt[b] | CC(t;3)[c] | EOMCC($P$) | CC($P$;$Q$) | EOMCC($P$) | CC($P$;$Q$) |
| 1.3 | −0.351 | 0.884 | 1.550 | 0.693 | 2.150 | 0.495 | 1.827 | 0.457 |
| 1.6 | −0.188 | 1.024 | 1.603 | 0.719 | 2.191 | 0.483 | 1.721 | 0.458 |
| 1.809[f] | 0.185 | 1.055 | 1.646 | 0.754 | 2.192 | 0.474 | 1.638 | 0.465 |
| 2.0 | 1.118 | 1.019 | 1.758 | 0.776 | 2.435 | 0.514 | 1.865 | 0.482 |
| 2.4 | 3.596 | 1.099 | 2.001 | 0.909 | 2.461 | 0.712 | 2.058 | 0.610 |
| 2.8 | 4.501 | 1.163 | 1.915 | 1.005 | 2.330 | 0.873 | 1.711 | 0.705 |
| 3.2 | 4.653 | 1.176 | 1.801 | 1.043 | 2.061 | 0.959 | 1.469 | 0.738 |
| 3.6 | 4.488 | 1.208 | 1.740 | 1.093 | 1.801 | 1.031 | 1.272 | 0.727 |
| 4.0 | 4.166 | 1.263 | 1.716 | 1.133 | 1.710 | 1.046 | 1.131 | 0.708 |
| 4.2 | 3.977 | 1.294 | 1.713 | 1.153 | 1.681 | 1.067 | 1.104 | 0.712 |
| 4.4 | 3.783 | 1.326 | 1.714 | 1.184 | 1.660 | 1.066 | 1.053 | 0.708 |

[a] CR-EOMCC(2,3) calculations.
[b] EOMCCSDt calculations using the active space consisting of the three highest occupied and two lowest unoccupied RHF orbitals.
[c] CC(t;3) calculations using the active space consisting of the three highest occupied and two lowest unoccupied RHF orbitals.
[d] EOMCC($P$) and CC($P$;$Q$) calculations using $P$ spaces consisting of all singly and doubly excited determinants and 1% of triply excited determinants identified by the adaptive CC($P$;$Q$) algorithm.
[e] EOMCC($P$) and CC($P$;$Q$) calculations using $P$ spaces consisting of all singly and doubly excited determinants and 2% of triply excited determinants identified by the adaptive CC($P$;$Q$) algorithm.
[f] The equilibrium value of the O–H bond length in the ground electronic state of water, as obtained in Ref. [S1] using the CCSD/cc-pVTZ method.

**Table S5**
Same as Table S3 for the 1 $^3$A″ state.

| | | | | | %T = 1[d] | | %T = 2[e] | |
|---|---|---|---|---|---|---|---|---|
| $R_{\mathrm{OH}}$ | EOMCCSD | CR(2,3)[a] | EOMCCSDt[b] | CC(t;3)[c] | EOMCC($P$) | CC($P$;$Q$) | EOMCC($P$) | CC($P$;$Q$) |
| 1.3 | −0.325 | 0.887 | 1.545 | 0.722 | 2.427 | 0.679 | 2.012 | 0.595 |
| 1.6 | −0.205 | 1.088 | 1.596 | 0.730 | 2.175 | 0.658 | 1.893 | 0.624 |
| 1.809[f] | 0.046 | 1.110 | 1.641 | 0.716 | 2.537 | 0.728 | 2.029 | 0.636 |
| 2.0 | 0.757 | 0.999 | 1.732 | 0.669 | 2.650 | 0.777 | 2.370 | 0.724 |
| 2.4 | 3.847 | 0.663 | 1.957 | 0.532 | 3.621 | 0.764 | 3.151 | 0.696 |
| 2.8 | 7.203 | 0.326 | 1.890 | 0.490 | 4.063 | 0.771 | 3.147 | 0.666 |
| 3.2 | 10.310 | −0.213 | 1.721 | 0.517 | 4.246 | 0.874 | 2.851 | 0.679 |
| 3.6 | 13.094 | −0.899 | 1.598 | 0.566 | 3.869 | 1.088 | 2.535 | 0.728 |
| 4.0 | 15.388 | −1.594 | 1.533 | 0.621 | 3.407 | 0.988 | 2.025 | 0.653 |
| 4.2 | 16.323 | −1.909 | 1.518 | 0.648 | 3.377 | 1.035 | 1.923 | 0.670 |
| 4.4 | 17.120 | −2.192 | 1.510 | 0.687 | 3.231 | 1.033 | 1.791 | 0.645 |

[a] CR-EOMCC(2,3) calculations.
[b] EOMCCSDt calculations using the active space consisting of the three highest occupied and two lowest unoccupied RHF orbitals.
[c] CC(t;3) calculations using the active space consisting of the three highest occupied and two lowest unoccupied RHF orbitals.
[d] EOMCC($P$) and CC($P$;$Q$) calculations using $P$ spaces consisting of all singly and doubly excited determinants and 1% of triply excited determinants identified by the adaptive CC($P$;$Q$) algorithm.
[e] EOMCC($P$) and CC($P$;$Q$) calculations using $P$ spaces consisting of all singly and doubly excited determinants and 2% of triply excited determinants identified by the adaptive CC($P$;$Q$) algorithm.
[f] The equilibrium value of the O–H bond length in the ground electronic state of water, as obtained in Ref. [S1] using the CCSD/cc-pVTZ method.

**Table S6**
Same as Table S3 for the 1 $^1$A′ state.

| | | | | | %T = 1[d] | | %T = 2[e] | |
|---|---|---|---|---|---|---|---|---|
| $R_{\mathrm{OH}}$ | EOMCCSD | CR(2,3)[a] | EOMCCSDt[b] | CC(t;3)[c] | EOMCC($P$) | CC($P$;$Q$) | EOMCC($P$) | CC($P$;$Q$) |
| 1.3 | −0.018 | 0.964 | 1.466 | 0.660 | 2.364 | 0.472 | 1.092 | 0.435 |
| 1.6 | 0.298 | 1.129 | 1.495 | 0.695 | 2.455 | 0.475 | 1.918 | 0.418 |
| 1.809[f] | 0.890 | 1.189 | 1.530 | 0.706 | 2.676 | 0.520 | 1.984 | 0.478 |
| 2.0 | 1.950 | 1.147 | 1.599 | 0.691 | 3.053 | 0.547 | 2.369 | 0.518 |
| 2.4 | 5.922 | 0.781 | 1.829 | 0.545 | 4.025 | 0.434 | 3.117 | 0.407 |
| 2.8 | 10.351 | 0.088 | 1.853 | 0.489 | 4.809 | 0.490 | 3.282 | 0.467 |
| 3.2 | 14.047 | −0.790 | 1.718 | 0.462 | 5.056 | 0.632 | 3.147 | 0.504 |
| 3.6 | 17.027 | −1.737 | 1.596 | 0.501 | 4.533 | 0.746 | 2.656 | 0.540 |
| 4.0 | 19.348 | −2.649 | 1.527 | 0.551 | 3.678 | 0.695 | 2.258 | 0.575 |
| 4.2 | 20.261 | −3.063 | 1.509 | 0.578 | 3.414 | 0.734 | 2.070 | 0.561 |
| 4.4 | 21.024 | −3.448 | 1.499 | 0.600 | 3.296 | 0.744 | 1.915 | 0.532 |

[a] CR-EOMCC(2,3) calculations.
[b] EOMCCSDt calculations using the active space consisting of the three highest occupied and two lowest unoccupied RHF orbitals.
[c] CC(t;3) calculations using the active space consisting of the three highest occupied and two lowest unoccupied RHF orbitals.
[d] EOMCC($P$) and CC($P$;$Q$) calculations using $P$ spaces consisting of all singly and doubly excited determinants and 1% of triply excited determinants identified by the adaptive CC($P$;$Q$) algorithm.
[e] EOMCC($P$) and CC($P$;$Q$) calculations using $P$ spaces consisting of all singly and doubly excited determinants and 2% of triply excited determinants identified by the adaptive CC($P$;$Q$) algorithm.
[f] The equilibrium value of the O–H bond length in the ground electronic state of water, as obtained in Ref. [S1] using the CCSD/cc-pVTZ method.

**Table S7**
Same as Table S3 for the 2 $^3$A′ state.

| | | | | | %T = 1[d] | | %T = 2[e] | |
|---|---|---|---|---|---|---|---|---|
| $R_{\mathrm{OH}}$ | EOMCCSD | CR(2,3)[a] | EOMCCSDt[b] | CC(t;3)[c] | EOMCC($P$) | CC($P$;$Q$) | EOMCC($P$) | CC($P$;$Q$) |
| 1.3 | −0.930 | 0.877 | 1.291 | 0.705 | 2.160 | 0.529 | 2.026 | 0.538 |
| 1.6 | −0.057 | 0.950 | 1.545 | 0.708 | 2.159 | 0.523 | 1.989 | 0.506 |
| 1.809[f] | 0.958 | 1.006 | 1.781 | 0.733 | 2.488 | 0.593 | 2.008 | 0.545 |
| 2.0 | 1.669 | 1.122 | 1.913 | 0.781 | 2.878 | 0.742 | 2.478 | 0.637 |
| 2.4 | 4.621 | 0.995 | 2.117 | 0.722 | 3.750 | 0.729 | 2.898 | 0.656 |
| 2.8 | 8.219 | 0.352 | 1.961 | 0.545 | 4.360 | 0.585 | 3.051 | 0.540 |
| 3.2 | 11.561 | −0.328 | 1.750 | 0.524 | 4.423 | 0.660 | 2.913 | 0.533 |
| 3.6 | 14.620 | −1.109 | 1.608 | 0.551 | 4.030 | 0.739 | 2.389 | 0.519 |
| 4.0 | 17.204 | −1.892 | 1.531 | 0.591 | 3.674 | 0.741 | 2.059 | 0.462 |
| 4.2 | 18.274 | −2.253 | 1.510 | 0.612 | 3.555 | 0.769 | 1.918 | 0.450 |
| 4.4 | 19.197 | −2.590 | 1.497 | 0.632 | 3.695 | 0.701 | 1.818 | 0.439 |

[a] CR-EOMCC(2,3) calculations.
[b] EOMCCSDt calculations using the active space consisting of the three highest occupied and two lowest unoccupied RHF orbitals.
[c] CC(t;3) calculations using the active space consisting of the three highest occupied and two lowest unoccupied RHF orbitals.
[d] EOMCC($P$) and CC($P$;$Q$) calculations using $P$ spaces consisting of all singly and doubly excited determinants and 1% of triply excited determinants identified by the adaptive CC($P$;$Q$) algorithm.
[e] EOMCC($P$) and CC($P$;$Q$) calculations using $P$ spaces consisting of all singly and doubly excited determinants and 2% of triply excited determinants identified by the adaptive CC($P$;$Q$) algorithm.
[f] The equilibrium value of the O–H bond length in the ground electronic state of water, as obtained in Ref. [S1] using the CCSD/cc-pVTZ method.

**Table S8**
Same as Table S3 for the 2 $^3$A$''$ state.

| $R_{\mathrm{OH}}$ | EOMCCSD | CR(2,3)[a] | EOMCCSDt[b] | CC(t;3)[c] | %T = 1[d] EOMCC($P$) | %T = 1[d] CC($P$;$Q$) | %T = 2[e] EOMCC($P$) | %T = 2[e] CC($P$;$Q$) |
|---|---|---|---|---|---|---|---|---|
| 1.3 | −0.547 | 0.933 | 1.370 | 0.736 | 2.392 | 0.726 | 2.314 | 0.655 |
| 1.6 | 0.286 | 1.044 | 1.620 | 0.711 | 2.430 | 0.672 | 2.165 | 0.608 |
| 1.809[f] | 1.181 | 1.049 | 1.825 | 0.679 | 2.808 | 0.710 | 2.323 | 0.623 |
| 2.0 | 1.877 | 1.052 | 1.927 | 0.647 | 3.071 | 0.840 | 2.540 | 0.714 |
| 2.4 | 2.210 | 1.111 | 1.740 | 0.596 | 3.906 | 1.066 | 3.334 | 0.808 |
| 2.8 | 2.703 | 1.472 | 1.477 | 0.543 | 4.215 | 1.145 | 3.384 | 0.777 |
| 3.2 | 5.070 | 2.801 | 1.355 | 0.505 | 5.281 | 1.284 | 3.706 | 0.831 |
| 3.6 | 11.868 | 6.744 | 1.409 | 0.484 | 7.607 | 1.634 | 4.470 | 0.844 |
| 4.0 | 21.864 | 11.891 | 1.504 | 0.481 | 9.244 | 1.753 | 4.926 | 0.804 |
| 4.2 | 25.767 | 13.294 | 1.503 | 0.483 | 9.172 | 1.595 | 4.889 | 0.736 |
| 4.4 | 28.470 | 13.976 | 1.482 | 0.625 | 9.097 | 1.523 | 4.806 | 0.705 |

[a] CR-EOMCC(2,3) calculations.
[b] EOMCCSDt calculations using the active space consisting of the three highest occupied and two lowest unoccupied RHF orbitals.
[c] CC(t;3) calculations using the active space consisting of the three highest occupied and two lowest unoccupied RHF orbitals.
[d] EOMCC($P$) and CC($P$;$Q$) calculations using $P$ spaces consisting of all singly and doubly excited determinants and 1% of triply excited determinants identified by the adaptive CC($P$;$Q$) algorithm.
[e] EOMCC($P$) and CC($P$;$Q$) calculations using $P$ spaces consisting of all singly and doubly excited determinants and 2% of triply excited determinants identified by the adaptive CC($P$;$Q$) algorithm.
[f] The equilibrium value of the O–H bond length in the ground electronic state of water, as obtained in Ref. [S1] using the CCSD/cc-pVTZ method.

**Table S9**
Same as Table S3 for the 2 $^1$A$'$ state.

| $R_{\mathrm{OH}}$ | EOMCCSD | CR(2,3)[a] | EOMCCSDt[b] | CC(t;3)[c] | %T = 1[d] EOMCC($P$) | %T = 1[d] CC($P$;$Q$) | %T = 2[e] EOMCC($P$) | %T = 2[e] CC($P$;$Q$) |
|---|---|---|---|---|---|---|---|---|
| 1.3 | −0.720 | 0.865 | 1.300 | 0.679 | 2.302 | 0.473 | 2.069 | 0.477 |
| 1.6 | 0.014 | 0.918 | 1.509 | 0.663 | 2.197 | 0.400 | 1.830 | 0.405 |
| 1.809[f] | 0.920 | 0.908 | 1.677 | 0.643 | 2.655 | 0.446 | 1.908 | 0.414 |
| 2.0 | 1.886 | 0.872 | 1.785 | 0.627 | 2.819 | 0.433 | 2.219 | 0.464 |
| 2.4 | 5.132 | 1.267 | 1.853 | 0.772 | 4.413 | 0.597 | 3.264 | 0.533 |
| 2.8 | 11.838 | 0.215 | 1.896 | 0.892 | 3.710 | 0.786 | 2.598 | 0.611 |
| 3.2 | 18.528 | −2.178 | 2.218 | 0.868 | 3.149 | 0.999 | 2.364 | 0.656 |
| 3.6 | 25.315 | −4.968 | 2.706 | 0.743 | 3.299 | 1.109 | 2.405 | 0.753 |
| 4.0 | 30.370 | −6.883 | 3.185 | 0.743 | 3.606 | 1.101 | 2.504 | 0.912 |
| 4.2 | 31.801 | −7.063 | 3.377 | 0.646 | 3.653 | 1.161 | 2.440 | 0.841 |
| 4.4 | 32.540 | −6.732 | 3.531 | 0.621 | 3.722 | 1.090 | 2.353 | 0.731 |

[a] CR-EOMCC(2,3) calculations.
[b] EOMCCSDt calculations using the active space consisting of the three highest occupied and two lowest unoccupied RHF orbitals.
[c] CC(t;3) calculations using the active space consisting of the three highest occupied and two lowest unoccupied RHF orbitals.
[d] EOMCC($P$) and CC($P$;$Q$) calculations using $P$ spaces consisting of all singly and doubly excited determinants and 1% of triply excited determinants identified by the adaptive CC($P$;$Q$) algorithm.
[e] EOMCC($P$) and CC($P$;$Q$) calculations using $P$ spaces consisting of all singly and doubly excited determinants and 2% of triply excited determinants identified by the adaptive CC($P$;$Q$) algorithm.
[f] The equilibrium value of the O–H bond length in the ground electronic state of water, as obtained in Ref. [S1] using the CCSD/cc-pVTZ method.

**Table S10**
Same as Table S3 for the 2 $^1$A$''$ state.

| | | | | | %T = 1[d] | | %T = 2[e] | |
|---|---|---|---|---|---|---|---|---|
| $R_{\text{OH}}$ | EOMCCSD | CR(2,3)[a] | EOMCCSDt[b] | CC(t;3)[c] | EOMCC($P$) | CC($P$;$Q$) | EOMCC($P$) | CC($P$;$Q$) |
| 1.3 | −0.688 | 0.912 | 1.340 | 0.722 | 2.153 | 0.702 | 2.209 | 0.624 |
| 1.6 | −0.078 | 0.963 | 1.582 | 0.684 | 2.202 | 0.607 | 2.049 | 0.583 |
| 1.809[f] | 0.649 | 0.905 | 1.776 | 0.642 | 2.565 | 0.652 | 2.171 | 0.593 |
| 2.0 | 1.252 | 0.845 | 1.875 | 0.604 | 2.685 | 0.777 | 2.465 | 0.686 |
| 2.4 | 1.371 | 0.776 | 1.717 | 0.562 | 3.247 | 0.890 | 2.886 | 0.701 |
| 2.8 | 1.147 | 0.846 | 1.483 | 0.523 | 3.039 | 0.805 | 2.577 | 0.578 |
| 3.2 | 1.309 | 1.103 | 1.348 | 0.493 | 3.586 | 0.790 | 2.588 | 0.588 |
| 3.6 | 2.177 | 1.642 | 1.289 | 0.473 | 3.757 | 0.783 | 2.493 | 0.544 |
| 4.0 | 4.156 | 2.805 | 1.274 | 0.461 | 4.680 | 1.140 | 2.823 | 0.734 |
| 4.2 | 5.598 | 3.693 | 1.277 | 0.459 | 4.871 | 1.217 | 2.820 | 0.637 |
| 4.4 | 7.284 | 4.759 | 1.283 | 0.460 | 5.282 | 1.208 | 2.800 | 0.098 |

[a] CR-EOMCC(2,3) calculations.
[b] EOMCCSDt calculations using the active space consisting of the three highest occupied and two lowest unoccupied RHF orbitals.
[c] CC(t;3) calculations using the active space consisting of the three highest occupied and two lowest unoccupied RHF orbitals.
[d] EOMCC($P$) and CC($P$;$Q$) calculations using $P$ spaces consisting of all singly and doubly excited determinants and 1% of triply excited determinants identified by the adaptive CC($P$;$Q$) algorithm.
[e] EOMCC($P$) and CC($P$;$Q$) calculations using $P$ spaces consisting of all singly and doubly excited determinants and 2% of triply excited determinants identified by the adaptive CC($P$;$Q$) algorithm.
[f] The equilibrium value of the O–H bond length in the ground electronic state of water, as obtained in Ref. [S1] using the CCSD/cc-pVTZ method.

**Table S11**
Same as Table S3 for the 3 $^3$A$''$ state.

| | | | | | %T = 1[d] | | %T = 2[e] | |
|---|---|---|---|---|---|---|---|---|
| $R_{\text{OH}}$ | EOMCCSD | CR(2,3)[a] | EOMCCSDt[b] | CC(t;3)[c] | EOMCC($P$) | CC($P$;$Q$) | EOMCC($P$) | CC($P$;$Q$) |
| 1.3 | 0.779 | 1.263 | 1.977 | 0.604 | 2.175 | 0.807 | 2.001 | 0.699 |
| 1.6 | 1.104 | 1.518 | 2.431 | 0.662 | 2.645 | 0.864 | 2.261 | 0.735 |
| 1.809[f] | 1.241 | 1.660 | 2.825 | 0.663 | 2.800 | 1.019 | 2.330 | 0.823 |
| 2.0 | 1.399 | 1.643 | 3.427 | 0.557 | 3.421 | 1.199 | 2.768 | 0.962 |
| 2.4 | 3.843 | 2.230 | 5.071 | 0.322 | 4.367 | 2.134 | 3.916 | 1.551 |
| 2.8 | 62.239 | 37.018 | 2.134 | 0.133 | 25.551 | 6.740 | 12.680 | 2.195 |
| 3.2 | 65.442 | 6.569 | 2.247 | 0.531 | 14.778 | 2.541 | 8.348 | 1.144 |
| 3.6 | 53.786 | −0.457 | 1.909 | 0.511 | 10.641 | 1.780 | 6.420 | 0.852 |
| 4.0 | 42.844 | −4.801 | 1.606 | 0.741 | 7.891 | 1.486 | 4.998 | 0.678 |
| 4.2 | 39.743 | −5.151 | 1.522 | 0.737 | 7.713 | 1.491 | 4.603 | 0.665 |
| 4.4 | 38.464 | −4.513 | 1.470 | 0.496 | 7.241 | 1.373 | 4.380 | 0.623 |

[a] CR-EOMCC(2,3) calculations.
[b] EOMCCSDt calculations using the active space consisting of the three highest occupied and two lowest unoccupied RHF orbitals.
[c] CC(t;3) calculations using the active space consisting of the three highest occupied and two lowest unoccupied RHF orbitals.
[d] EOMCC($P$) and CC($P$;$Q$) calculations using $P$ spaces consisting of all singly and doubly excited determinants and 1% of triply excited determinants identified by the adaptive CC($P$;$Q$) algorithm.
[e] EOMCC($P$) and CC($P$;$Q$) calculations using $P$ spaces consisting of all singly and doubly excited determinants and 2% of triply excited determinants identified by the adaptive CC($P$;$Q$) algorithm.
[f] The equilibrium value of the O–H bond length in the ground electronic state of water, as obtained in Ref. [S1] using the CCSD/cc-pVTZ method.

**Table S12**
Same as Table S3 for the 3 $^1$A′ state.

| | | | | | %T = 1[d] | | %T = 2[e] | |
|---|---|---|---|---|---|---|---|---|
| $R_{OH}$ | EOMCCSD | CR(2,3)[a] | EOMCCSDt[b] | CC(t;3)[c] | EOMCC(*P*) | CC(*P*;*Q*) | EOMCC(*P*) | CC(*P*;*Q*) |
| 1.3 | 1.189 | 1.471 | 1.698 | 0.995 | 2.737 | 0.526 | 2.168 | 0.425 |
| 1.6 | 1.674 | 1.605 | 1.820 | 1.052 | 2.551 | 0.534 | 2.005 | 0.497 |
| 1.809[f] | 2.399 | 1.598 | 1.870 | 1.042 | 2.741 | 0.624 | 1.855 | 0.513 |
| 2.0 | 3.392 | 1.517 | 1.874 | 1.010 | 3.087 | 0.770 | 2.392 | 0.631 |
| 2.4 | 5.272 | 0.714 | 1.659 | 0.795 | 4.087 | 0.584 | 3.029 | 0.482 |
| 2.8 | 6.462 | 0.852 | 1.586 | 0.684 | 3.981 | 0.571 | 2.994 | 0.525 |
| 3.2 | 12.832 | 2.422 | 1.712 | 0.742 | 5.674 | 1.479 | 3.886 | 0.732 |
| 3.6 | 23.485 | 5.089 | 1.782 | 0.676 | 7.575 | 1.980 | 4.353 | 0.674 |
| 4.0 | 29.845 | 5.471 | 1.661 | 0.449 | 8.569 | 2.733 | 4.717 | 1.418 |
| 4.2 | 30.434 | 3.564 | 1.493 | 0.643 | 7.649 | 1.735 | 3.591 | 0.561 |
| 4.4 | 32.035 | 2.203 | 1.411 | 0.754 | 8.006 | 1.133 | 3.338 | 0.612 |

[a] CR-EOMCC(2,3) calculations.
[b] EOMCCSDt calculations using the active space consisting of the three highest occupied and two lowest unoccupied RHF orbitals.
[c] CC(t;3) calculations using the active space consisting of the three highest occupied and two lowest unoccupied RHF orbitals.
[d] EOMCC(*P*) and CC(*P*;*Q*) calculations using *P* spaces consisting of all singly and doubly excited determinants and 1% of triply excited determinants identified by the adaptive CC(*P*;*Q*) algorithm.
[e] EOMCC(*P*) and CC(*P*;*Q*) calculations using *P* spaces consisting of all singly and doubly excited determinants and 2% of triply excited determinants identified by the adaptive CC(*P*;*Q*) algorithm.
[f] The equilibrium value of the O–H bond length in the ground electronic state of water, as obtained in Ref. [S1] using the CCSD/cc-pVTZ method.

**Table S13**
Same as Table S3 for the 3 $^3$A′ state.

| | | | | | %T = 1[d] | | %T = 2[e] | |
|---|---|---|---|---|---|---|---|---|
| $R_{OH}$ | EOMCCSD | CR(2,3)[a] | EOMCCSDt[b] | CC(t;3)[c] | EOMCC(*P*) | CC(*P*;*Q*) | EOMCC(*P*) | CC(*P*;*Q*) |
| 1.3 | 0.720 | 1.272 | 1.929 | 0.985 | 2.377 | 0.498 | 1.910 | 0.414 |
| 1.6 | 1.352 | 1.531 | 1.980 | 1.066 | 2.595 | 0.625 | 2.005 | 0.558 |
| 1.809[f] | 2.074 | 1.592 | 1.991 | 1.045 | 2.694 | 0.734 | 1.933 | 0.572 |
| 2.0 | 2.950 | 1.393 | 2.060 | 0.923 | 3.051 | 0.732 | 2.542 | 0.629 |
| 2.4 | 3.158 | 0.986 | 1.760 | 0.674 | 3.907 | 0.704 | 3.037 | 0.618 |
| 2.8 | 4.223 | 1.175 | 1.541 | 0.726 | 3.931 | 0.702 | 2.879 | 0.580 |
| 3.2 | 6.986 | 1.528 | 1.452 | 0.772 | 4.083 | 0.799 | 2.817 | 0.580 |
| 3.6 | 11.320 | 2.330 | 1.412 | 0.802 | 4.111 | 1.203 | 2.793 | 0.676 |
| 4.0 | 16.730 | 3.829 | 1.379 | 0.800 | 4.471 | 1.611 | 3.003 | 0.858 |
| 4.2 | 19.566 | 5.000 | 1.363 | 0.777 | 4.984 | 1.847 | 3.134 | 0.958 |
| 4.4 | 22.282 | 6.656 | 1.348 | 0.826 | 5.525 | 2.073 | 3.323 | 0.996 |

[a] CR-EOMCC(2,3) calculations.
[b] EOMCCSDt calculations using the active space consisting of the three highest occupied and two lowest unoccupied RHF orbitals.
[c] CC(t;3) calculations using the active space consisting of the three highest occupied and two lowest unoccupied RHF orbitals.
[d] EOMCC(*P*) and CC(*P*;*Q*) calculations using *P* spaces consisting of all singly and doubly excited determinants and 1% of triply excited determinants identified by the adaptive CC(*P*;*Q*) algorithm.
[e] EOMCC(*P*) and CC(*P*;*Q*) calculations using *P* spaces consisting of all singly and doubly excited determinants and 2% of triply excited determinants identified by the adaptive CC(*P*;*Q*) algorithm.
[f] The equilibrium value of the O–H bond length in the ground electronic state of water, as obtained in Ref. [S1] using the CCSD/cc-pVTZ method.
